# Supplementary material for: Modeling financial transactions via random walks on temporal networks
Source: arXiv:2602.20713 ancillary file (2026-02-24)
Supplement: Supplementary file 1 [file SM.pdf]

Supplementary Material:

# Modeling financial transactions via random walks on temporal networks

Carolina E. Mattsson,[1] Claudio Cellerini,[2] Jaume Ojer,[3] and Michele Starnini[4]

[1]*Innovation Advisory, Intesa Sanpaolo, 10138 Torino, Italy*

[2]*Department of Physics, Universitá di Torino, 10125 Torino, Italy*

[3]*Institut de Física Interdisciplinària i Sistemes Complexos (IFISC, CSIC-UIB), 07122 Palma de Mallorca, Spain*

[4]*Department of Engineering, Universitat Pompeu Fabra, 08018 Barcelona, Spain*

## I. ANALYTICAL SOLUTION OF THE MODEL

### A. Model definition

We consider a network composed of $N$ nodes, where each node $i$ is uniquely characterized by three continuous features:

- **Activity rate ($a_i$):** $a_i \in [a_{\min}, a_{\max}]$, where $a_{\min} \ll 1$. Each node $i$ activates independently following a Poisson process with rate $a_i$.
- **Attractiveness ($b_i$):** $b_i \in [b_{\min}, b_{\max}]$, where $b_{\min} \ll 1$. When a node $i$ activates, it forms a directed link to another node $j$. The probability of choosing node $j$ as a destination is proportional to its attractiveness $b_j$.
- **Spending rate ($s_i$):** $s_i \in [s_{\min}, s_{\max}]$, where $s_{\min} \ll 1$. This governs the random walker's movement, which jumps from the source node $i$ to the destination node $j$ with probability $s_i$.

The random walker dynamics is defined as follows: A random walker (RW) arriving at node $i$ at time $t$ waits for node $i$ to activate. Node $i$ activates at some $t' > t$ by sending a single link to a chosen node $j$ (chosen with probability proportional to $b_j$). The RW then jumps from node $i$ to node $j$ with probability $s_i$. If the RW does not jump (with probability $1 - s_i$), it remains at node $i$ and waits for the next activation event of node $i$. We consider $M$ independent RWs on this network. This is the basic formulation of the model, dubbed the **Binomial model**.

A key modification can be introduced regarding the jump process. Instead of a fixed jump probability $s_i$ for each individual jump attempt (given an activation event), the number of RWs jumping from node $i$ is now governed by a Beta-Binomial distribution. For node $i$, the mean of the underlying Beta distribution is equal to $s_i$, and the sample size/precision parameter is a

fixed global value $\xi$ independent of the nodes. We dub this modification the **Beta-Binomial model**.

We assume the features $a$, $b$, and $s$ are distributed according to their respective probability density functions (PDFs): $f(a)$, $g(b)$, and $h(s)$. The variables $a$ and $b$ may be correlated, while $s$ is assumed to be independent of $a$ and $b$. Thus, the joint PDF of a node having features $(a, b, s)$ is $F(a, b, s) = P(a, b)\, h(s)$.

### B. Derivation of the stationary probability

We aim to find the stationary probability $\pi_{a,b,s}$ of finding a single RW on a node characterized by specific features $(a, b, s)$.

The transition rate at which a RW jumps from a source node $i$ to a destination node $j$, $W_{ij}$, depends on the source node's activation rate, $a_i$, and its effective jump probability, $s_i$. The destination node $j$ is chosen with probability proportional to its attractiveness, $b_j$. Thus, the transition rate is

$$W_{ij} = a_i s_i \frac{b_j}{\sum_k b_k}. \tag{1}$$

Let $p_j(t)$ be the probability that the RW is at node $j$ at time $t$. The continuous-time master equation for $p_j(t)$ is

$$\frac{dp_j(t)}{dt} = \sum_i p_i(t) W_{ij} - \sum_k p_j(t) W_{jk}. \tag{2}$$

In the stationary state, the time derivative is zero, leading to

$$\sum_i \pi_i W_{ij} = \sum_k \pi_j W_{jk}, \tag{3}$$

where $\pi_j$ is the stationary probability for the RW to be at node $j$. Substituting from Eq. (1), we obtain

$$\sum_i \pi_i a_i s_i \frac{b_j}{\sum_k b_k} = \pi_j a_j s_j. \tag{4}$$

Thus,

$$\pi_j = \frac{\mu\, b_j}{a_j s_j}, \tag{5}$$

where $\mu \equiv \frac{\sum_i \pi_i a_i s_i}{\sum_k b_k}$. By normalizing $\sum_j \pi_j = 1$, we find

$$\mu = \frac{1}{\sum_k \frac{b_k}{a_k s_k}}, \tag{6}$$

which leads to

$$\pi_j = \frac{\frac{b_j}{a_j s_j}}{\sum_k \frac{b_k}{a_k s_k}}. \tag{7}$$

That is, the stationary probability of finding the RW at node $j$ is proportional to its attractiveness $b_j$, and inversely proportional to its activity $a_j$ and spending rate $s_j$. In the limit of large $N$, the stationary probability $\pi_{a,b,s}$ reads as

$$\pi_{a,b,s} = \frac{1}{N\langle b/a\rangle_P \, \langle s^{-1}\rangle_h} \frac{b}{as}, \tag{8}$$

where $\langle \ldots \rangle_P$ and $\langle \ldots \rangle_h$ denote the mean value computed from the distribution $P(a,b)$ and $h(s)$, respectively.

It is worth stressing that the stationary probability $\pi_{a,b,s}$ is determined by the balance of average incoming and outgoing rates in the master equation, see Eq. (3). Since the transition rate $W_{ij}$ is defined by Eq. (1) for both the Binomial model and the Beta-Binomial model, the stationary probability given by Eq. (8) is also identical for both models.

### C. Probability distribution of walkers on the network

We are interested in $P(m)$, the probability of finding $m$ RWs present on a randomly chosen node in the network, in the stationary state. The general equation for $P(m)$ reads

$$P(m) = \int_{a_{\min}}^{a_{\max}} \int_{b_{\min}}^{b_{\max}} \int_{s_{\min}}^{s_{\max}} p(m \mid a,b,s)\, F(a,b,s)\, da\, db\, ds. \tag{9}$$

On a static network with $M$ independent RWs, the probability of finding $m$ RWs on a node with specific features $(a,b,s)$ follows a binomial distribution, $p(m \mid a,b,s) = \mathrm{Bin}\,(M, \pi_{a,b,s})$. If $M$ is large and $\pi_{a,b,s}$ is sufficiently small, we can approximate the binomial distribution as a Poisson distribution, i.e., $p(m \mid a,b,s) = \mathrm{Pois}\,(\lambda_{a,b,s})$, where

$$\lambda_{a,b,s} = M\pi_{a,b,s} = K_0 \frac{b}{as} \tag{10}$$

is the expected value or mean, with $K_0 \equiv \frac{M}{N\langle b/a\rangle_P \, \langle s^{-1}\rangle_h}$. Figure 1(a)-(c) shows $\lambda_{a,b,s}$ as a function of $(a,b,s)$ in the Binomial model, confirming that the stationary probability $\pi_{a,b,s}$ is proportional to $b$ and inversely proportional to $a$ and $s$. On the other hand, Figure 1(d)-(f) shows $\lambda_{a,b,s}$ in the Beta-Binomial model with $\xi = 1$ (high dispersion). One can see that $\pi_{a,b,s}$ preserves the same dependency on features $(a,b,s)$ as in the simpler Binomial model. Therefore, Eq. (10) is valid for both Binomial and Beta-Binomial models.

In the following, we assume perfect correlation between activity and attractiveness, which means that the joint PDF of a node having features $(a,b,s)$ can be written as $F(a,b,s) =$

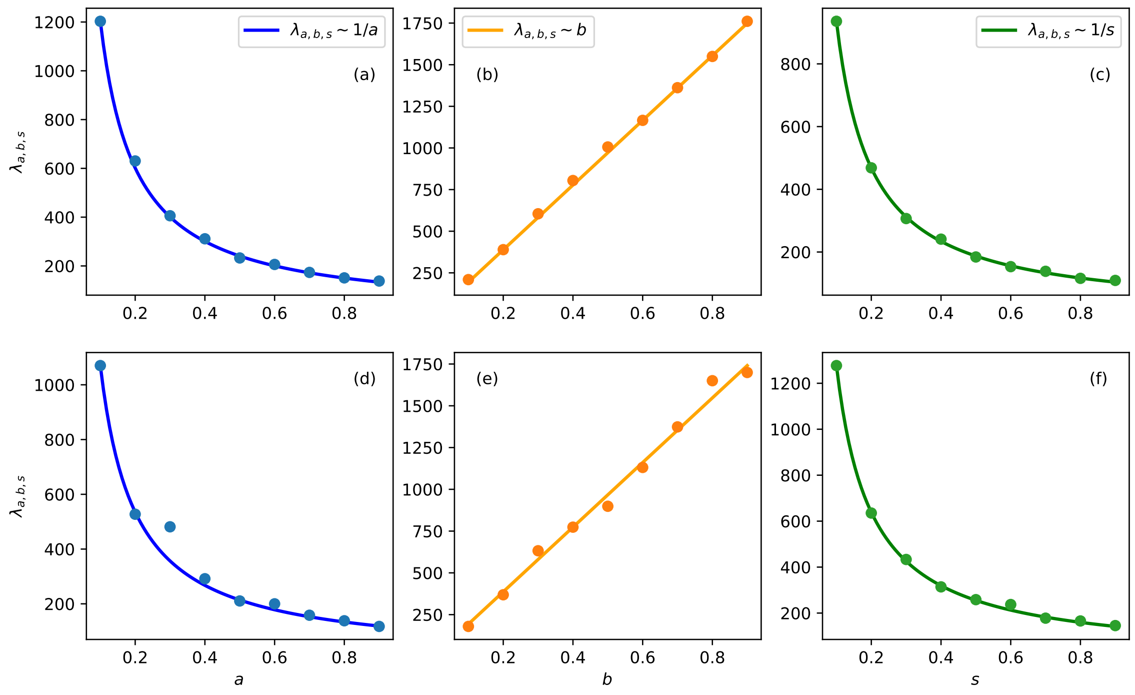


FIG. 1: Mean value $\lambda_{a,b,s}$ in the Binomial model [(a), (b), (c)] and the Beta-Binomial model with $\xi = 1$ [(d), (e), (f)], for different values of activity [(a), (d)], attractiveness [(b), (e)], and spending rate [(c), (f)]. Numerical simulations and theoretical prediction $\lambda_{a,b,s} \propto \frac{b}{as}$ are shown in points and solid lines, respectively.

$f(a)\,\delta(b-a)\,h(s)$. Therefore, Eq. (9) reduces to

$$P(m) = \int_{s_{\min}}^{s_{\max}} p(m \mid s)\, h(s)\, ds. \tag{11}$$

We will consider a generic power-law spending rate distribution of the form $h(s) \sim s^{\sigma}$. Note that the minimum spending rate in the population, $s_{\min}$, cannot go to zero to avoid a divergence in $\lambda_s$, see Eq. (10). Indeed, if a node has a zero spending rate, all RWs would never jump and would accumulate on that node. Without loss of generality, we define $s_{\min} = s_{\max}/N$, so we ensure that $s_{\min} \ll 1$.

On a temporal network, however, RWs do not move independently. While not interacting directly, they are coupled through the nodes' activity. Indeed, RWs accumulate on a given node until it activates, at which point each RW may jump with probability $s$. When the jump probability $s$ is large, RWs tend to jump together. In the limit of small $s$, instead, just a few RWs jump, and we recover the independence assumption. We will treat first the simpler small $s$ case, then for general $s$, and finally finite $\xi$.

### 1. *Limit of small s*

By using the Poisson approximation, $p(m \mid s) = \mathrm{Pois}(\lambda_s)$, from Eq. (11) we obtain

$$P(m) = \int_{s_{\min}}^{s_{\max}} \frac{(\lambda_s)^m \, e^{-\lambda_s}}{m!} \, h(s) \, ds \sim \frac{1}{m!} \int_{s_{\max}/N}^{s_{\max}} \left(\frac{K_0}{s}\right)^m e^{-\frac{K_0}{s}} \, s^{\sigma} \, ds. \tag{12}$$

Defining $u \equiv K_0/s$, we get

$$P(m) \sim \frac{1}{m!} \int_{K_0/s_{\max}}^{NK_0/s_{\max}} u^{m-\sigma-2} \, e^{-u} \, du, \tag{13}$$

which can be expressed in terms of the upper incomplete Gamma function $\Gamma(z,x) = \int_x^{\infty} t^{z-1} \, e^{-t} \, dt$ as [1]

$$P(m) \sim \frac{\Gamma\left(m-\sigma-1, K_0/s_{\max}\right) - \Gamma\left(m-\sigma-1, NK_0/s_{\max}\right)}{m!}. \tag{14}$$

For large $M$, the second term of the previous expression vanishes, leading to

$$P(m) \sim \frac{\Gamma\left(m-\sigma-1, K_0/s_{\max}\right)}{m!}. \tag{15}$$

*a. Limit of large m.* Note that, when $z \gg x$, we can approximate $\Gamma(z,x) = \Gamma(z)$, where $\Gamma(z) = \int_0^{\infty} t^{z-1} \, e^{-t} \, dt$ is the Gamma function. Therefore, for $m \gg K_0/s_{\max}$, Eq. (15) becomes

$$P(m) \sim \frac{\Gamma(m-\sigma-1)}{m!}. \tag{16}$$

If $\sigma \in \mathbb{Z}$, we have $\Gamma(m-\sigma-1) = (m-\sigma-2)!$, so Eq. (16) reduces to

$$P(m) \sim m^{-\nu}, \tag{17}$$

where $\nu \equiv \sigma + 2$.

While we obtained Eq. (17) in the limit of small $s$, we note that it is expected to be valid in any case, since the asymptotic behavior of $P(m)$ for large $m$ is determined by nodes with small $s$. Indeed, the mean number of RWs $\lambda_s$ is inversely proportional to $s$, so nodes with large $m$ have a small $s$. For these nodes, we can approximate $p(m \mid s)$ to a Poisson distribution. Therefore, Eq. (17) is valid for any distribution $h(s) \sim s^{\sigma}$, as long as the minimum $s_{\min}$ vanishes in the thermodynamic limit $N \to \infty$, which we previously imposed by defining $s_{\min} = s_{\max}/N$.

*b. Uniform case $\sigma = 0$.* In the case of uniform spending rate with $\sigma = 0$, its probability density function is simply $h(s) = \frac{1}{s_{\max} - s_{\min}}$, so $K_0/s_{\max} \approx \frac{M}{N \ln(N)}$ in the limit of large $N$. Under these conditions, Eq. (15) becomes

$$P(m) = \frac{M}{N \ln(N)} \frac{\Gamma\left(m-1, \frac{M}{N \ln(N)}\right)}{m!}. \tag{18}$$

Thus, we get the asymptotic behavior

$$P(m) \sim m^{-2} \tag{19}$$

for $m \gg \frac{M}{N \ln(N)}$, as expected from Eq. (17).

### *2. General s*

For non-vanishing values of $s$, RWs cannot be assumed independent, thus the conditional probability of finding $m$ RWs on a node with spending rate $s$, $p(m \mid s)$, is no longer a binomial distribution. When many RWs jump from a node, they all end up at the same destination, introducing correlation in their co-location. To model this correlation, we extend the binomial form of the $p(m \mid s)$ to a beta-binomial distribution, $\mathrm{BetaBin}(M, \alpha, \beta)$, with the same mean $\frac{M\alpha}{\alpha+\beta} = M\pi_s = \lambda_s$. This introduces a free parameter $r$ governing the correlation in RWs co-location, termed intra-class correlation in the statistics literature [2]. The parametrization recovering the required mean can be written as

$$p(m \mid s) = \mathrm{BetaBin}\left(M, \frac{r}{1-\lambda_s/M}, \frac{Mr}{\lambda_s}\right), \tag{20}$$

where $r$ is the free parameter accounting for the correlations induced by co-jumping and $\lim_{M\to\infty} \frac{r}{1-\lambda_s/M} = r$. To apply the Poisson approximation (i.e., large $M$ and sufficiently small $\pi_s$), we require the corresponding distributional limit of the beta-binomial distribution. The standard limit can be written as [3]

$$\lim_{M\to\infty} \mathrm{BetaBin}\left(M, r, \frac{M\,r}{\lambda_s}\right) = \mathrm{NB}\left(r, \frac{r}{r+\lambda_s}\right), \tag{21}$$

where $\mathrm{NB}\left(r, \frac{r}{r+\lambda_s}\right)$ is a negative binomial distribution also with mean $\lambda_s$, leading to

$$p(m \mid s) = \mathrm{NB}\left(r, \frac{r}{r+\lambda_s}\right). \tag{22}$$

Interestingly, the variance of the distribution $\mathrm{NB}\left(r, \frac{r}{r+\lambda_s}\right)$ is $\sigma^2_{\mathrm{NB}} = \sigma^2_{\mathrm{Pois}} + \lambda_s^2/r$, where $\sigma^2_{\mathrm{Pois}} = \lambda_s$ is the variance of the Poisson distribution. The excess variance $\lambda_s^2/r$ results from overdispersion due to average co-location correlations, which are encoded in the parameter $r$.

The parameter $r$ remains to be specified. Here we note that co-location correlations arise from RWs jumping together to the same destination. Since the recipient is chosen independently of $s$, the induced correlations should be uniform across nodes. Specifically, the beta-binomial intra-class correlation $\frac{1}{\alpha+\beta+1}$ [2] should be independent of $s$. For large $M$, we have $\alpha \approx r$ and $\alpha+\beta+1 = r + \frac{Mr}{\lambda_s} + 1 \approx \frac{Mr}{\lambda_s}$. Thus, the intra-class correlation becomes

$$\frac{1}{\alpha+\beta+1} \approx \frac{1}{N\,\langle s\rangle_h\, s\, r}, \tag{23}$$

where we used $\lambda_s = \frac{K_0}{s}$ and $K_0 = \frac{M}{N\,\langle s^{-1}\rangle_h}$ from Eq. 10. According to Eq. 23, we fix $r \propto 1/s$ to ensure that the underlying co-location correlations of the RWs do not depend on $s$. The parameter $r$ diverges for small $s$, recovering the Poisson distribution corresponding to the case without correlations, i.e., the independence assumption.

Having established $r \propto 1/s$, we specify $r = r_0/s$ and $r_0 \equiv 1 - \langle s \rangle_h$ such that

$$r = \frac{1 - \langle s \rangle_h}{s}, \tag{24}$$

which becomes $r = (1-s)/s$ in the homogeneous case $s_i = \langle s \rangle_h \; \forall i$. This reproduces the formula $r \approx 1/s - 1$ put forward in Ref. [4] regarding a relevant continuous wealth-exchange model, see the so-called A-2 model [5–7]. Thus, in this homogeneous case, our discrete model admits a simple interpretation of the expression: $(1-s)/s$ represents the ratio of the probability for RWs to stay on an activated node over their probability to jump.

Hence, Eq. (22) becomes

$$p(m \mid s) = \mathrm{NB}(r, p) = \frac{\Gamma(m+r)}{m!\,\Gamma(r)}\, p^r (1-p)^m, \tag{25}$$

where $r$ is given by Eq. (24) and

$$p = \frac{r}{r + \lambda_s} = \frac{1 - \langle s \rangle_h}{1 - \langle s \rangle_h + K_0} \tag{26}$$

is a constant independent of the spending rate $s$. Substituting Eq. (25) into Eq. (11), we have

$$\begin{aligned} P(m) &= \int_{s_{\min}}^{s_{\max}} \frac{\Gamma(m+r)}{m!\,\Gamma(r)}\, p^r (1-p)^m \, h(s)\, ds \\ &\sim \frac{1}{m!} \left( \frac{K_0}{1 - \langle s \rangle_h + K_0} \right)^m \int_{s_{\max}/N}^{s_{\max}} \frac{\Gamma\left(m + \frac{1-\langle s \rangle_h}{s}\right)}{\Gamma\left(\frac{1-\langle s \rangle_h}{s}\right)} \left( \frac{1 - \langle s \rangle_h}{1 - \langle s \rangle_h + K_0} \right)^{\frac{1-\langle s \rangle_h}{s}} s^{\sigma}\, ds. \end{aligned} \tag{27}$$

We evaluate this integral numerically, see Section I E.

*a. Overdispersion in the Beta-Binomial model.* The precision parameter $\xi$ in the Beta-Binomial model introduces correlation in the jump decisions of the RWs at an activated node. This further correlates co-presence at the next node, yielding additional overdispersion in node occupancy. Therefore, there are now two different sources of correlations: $r$, due to the average tendency for RWs to jump together, and $\xi$, due to correlation in jump decisions of RWs. Recall that the variance of $p(m \mid s) = \mathrm{NB}\left(r, \frac{r}{r+\lambda_s}\right)$ is $\sigma^2_{\mathrm{NB}} = \sigma^2_{\mathrm{Pois}} + \lambda_s^2/r$. If we denote the excess variance by $\sigma_r^2 = \lambda_s^2/r$, which accounts for average co-location correlations, we model the overall overdispersion under the Beta-Binomial model as $\sigma^2_{\mathrm{eff}} = \sigma_r^2 + \sigma_\xi^2$, that is

$$\frac{1}{r_{\mathrm{eff}}} = \frac{1}{r} + \frac{1}{\xi}. \tag{28}$$

Under these conditions, the conditional probability of observing $m$ RWs on a node with spending rate $s$ is $p(m \mid s, \xi) = \mathrm{NB}\left(r_{\mathrm{eff}}, \frac{r_{\mathrm{eff}}}{r_{\mathrm{eff}}+\lambda_s}\right)$, with $r_{\mathrm{eff}}$ given by Eq. (28). Thus, the distribution $P(m)$ reads

$$P(m) \sim \frac{1}{m!} \int_{s_{\max}/N}^{s_{\max}} \frac{\Gamma(m + r_{\mathrm{eff}})}{\Gamma(r_{\mathrm{eff}})} \frac{(r_{\mathrm{eff}})^{r_{\mathrm{eff}}}\, (\lambda_s)^m}{(r_{\mathrm{eff}} + \lambda_s)^{r_{\mathrm{eff}}+m}}\, s^{\sigma}\, ds. \tag{29}$$

We evaluate this integral numerically, see Section I E.

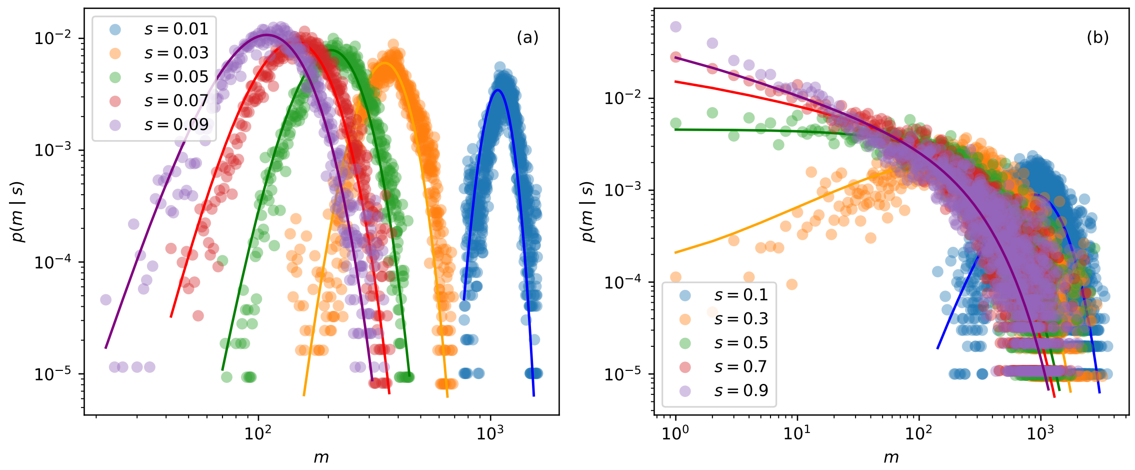


FIG. 2: Conditional probability $p(m \mid s)$ for different values of spending rate $s$ in the Binomial model, with $s_{\max} = 0.1$ (a) and $s_{\max} = 1.0$ (b). Solid lines correspond to negative binomial distributions, NB $\left(r, \frac{r}{r+\lambda_s}\right)$, where $r$ is given by Eq. (24) and $\lambda_s = K_0/s$. We used $N = 10^4$, $M = 10^7$, uniform spending rates, and perfect correlation between activity and attractiveness.

### *3. Comparison with numerical simulations*

We test our analytical approaches for both the small and general $s$ cases with numerical simulations of the Binomial model.

Figure 2 compares numerical simulations (points) against the conditional probability $p(m \mid s)$ given by Eq. (25) (solid lines) for two different values of $s_{\max}$. One can see that, while for small $s$ the conditional probability $p(m \mid s)$ is similar to a Poisson distribution, as soon as $s$ increases, $p(m \mid s)$ becomes very different from a Poissonian, especially for small values of $m$. In all cases, the extension to a negative binomial given by Eq. (25) is recovered with very good accuracy.

Figure 3 compares numerical simulations (points) against the distribution $P(m)$ for uniform spending rates ($\sigma = 0$) obtained numerically from Eq. (27) (solid lines), the analytical prediction given by Eq. (18) (gray line) under the independence assumption (i.e., small $s$), and the asymptotic behavior for large $m$ predicted by Eq. (19) (dashed line), for different values of $s_{\max}$. One can see that, for $m > K_0/s_{\max}$ (plotted as a dotted line), the asymptotic behavior $P(m) \sim m^{-2}$ is very well reproduced. This means that the power-law decay is valid also when large values of $s$ are sampled from the distribution $h(s)$. Indeed, nodes with small $s$ govern the regime $m > K_0/s_{\max}$, while nodes with large $s$ govern the regime $m < K_0/s_{\max}$. For this reason, the analytical prediction obtained under the independence assumption only works for $m > K_0/s_{\max}$. The whole $P(m)$ distribution, also for small values of $m$, is recovered with very good accuracy by a numerical integration of Eq. (27), for all values of $s_{\max}$.

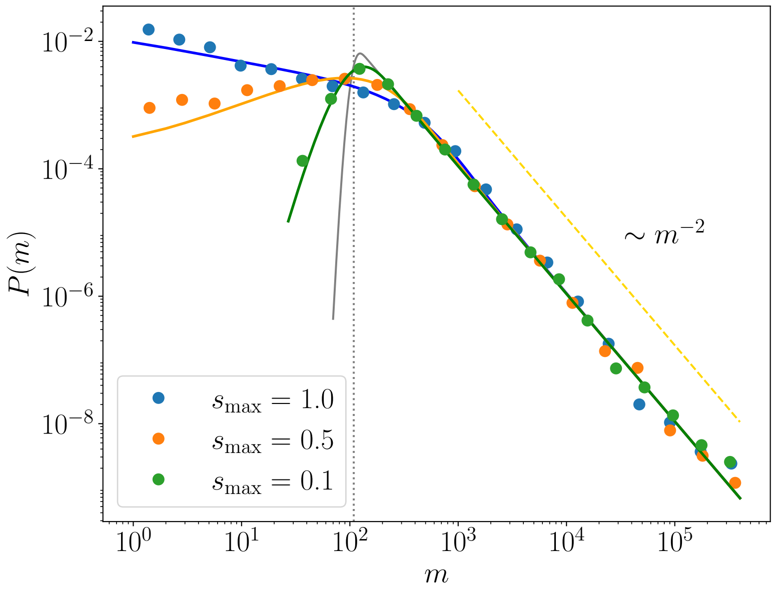


FIG. 3: Probability distribution $P(m)$ in the Binomial model for different values of maximum spending rate $s_{\max}$. Solid lines correspond to numerical integrations of Eq. (27). Gray line corresponds to the analytical solution of $P(m)$ obtained under the independence assumption, see Eq. (18). Yellow dashed line shows the predicted power-law scaling $P(m) \sim m^{-2}$, see Eq. (19). Vertical dotted line corresponds to $m = K_0/s_{\max} \approx \frac{M}{N \ln(N)}$. We used $N = 10^4$, $M = 10^7$, $\sigma = 0$, and perfect correlation between activity and attractiveness.

Figure 4 compares numerical simulations (points) against the distribution $P(m)$ for $s_{\max} = 0.1$ obtained numerically from Eq. (27) (solid lines) and the asymptotic behavior for large $m$ predicted by Eq. (17) (dashed lines), for different values of exponent $\sigma$. One can see that, for $m > K_0/s_{\max}$ (plotted as a dotted line), the asymptotic behavior $P(m) \sim m^{-(\sigma+2)}$ is very well reproduced. The whole $P(m)$ distribution, also for small values of $m$, is recovered with very good accuracy by a numerical integration of Eq. (27), for all values of $\sigma$.

In Fig. 1(a) of the main text, we show that our theoretical approach for $P(m)$ also works in the Beta-Binomial model with finite $\xi$, by integrating numerically Eq. (29).

### D. Probability distribution of jumping walkers

Now, we focus on $P(w)$, the probability of observing exactly $w$ RWs jumping during a randomly chosen activation event. $P(w)$ is obtained by averaging over all possible nodes and all possible numbers of RWs present on those nodes at the moment of their activation, $m$, weighted

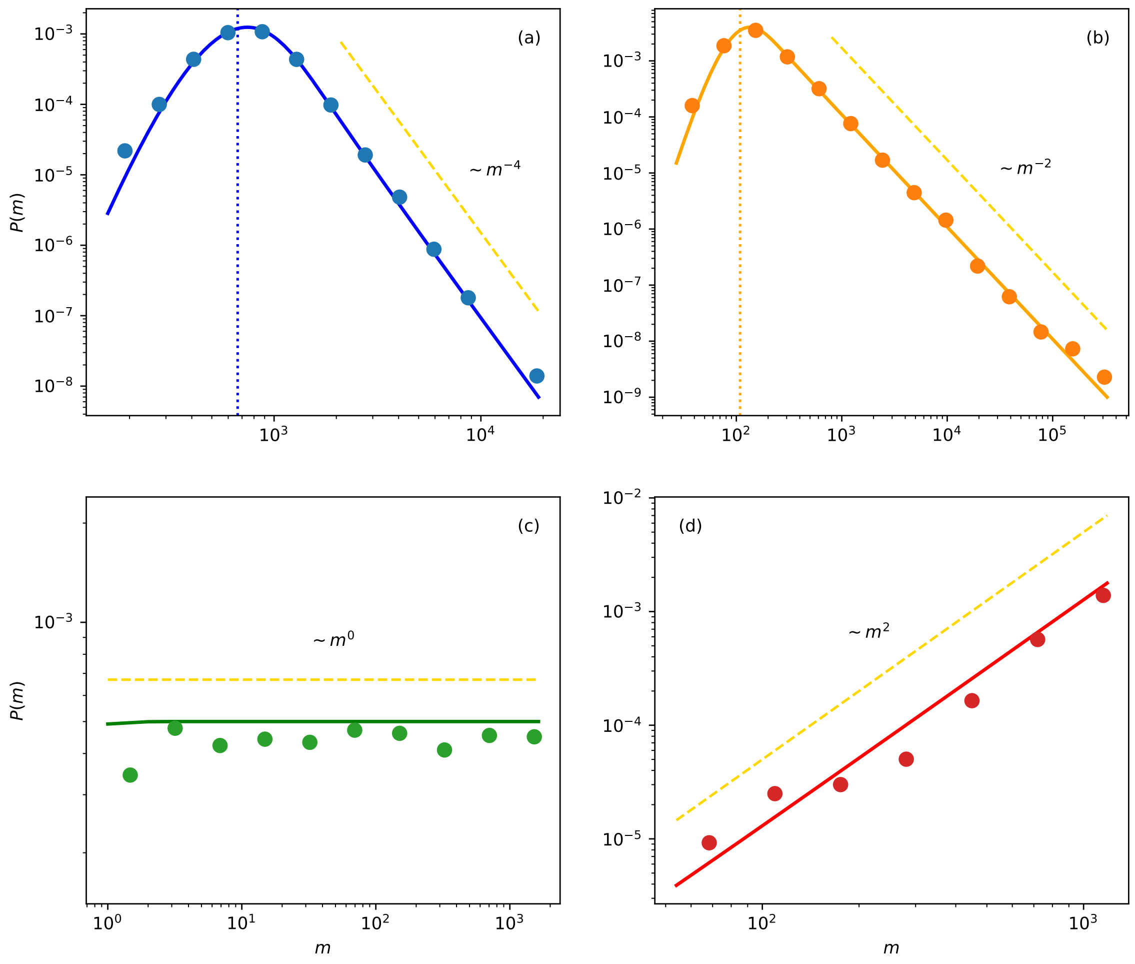


FIG. 4: Probability distribution $P(m)$ in the Binomial model for (a) $\sigma = 2$, (b) $\sigma = 0$, (c) $\sigma = -2$, and (d) $\sigma = -4$. Solid lines correspond to numerical integrations of Eq. (27). Yellow dashed lines show the predicted power-law scaling $P(m) \sim m^{-(\sigma+2)}$, see Eq. (17). Vertical dotted lines correspond to $m = K_0/s_{\max}$. Note that $K_0/s_{\max} < 1$ for $\sigma < 0$, so $P(m)$ behaves as a power-law across the full range of $m$. We used $N = 10^4$, $M = 10^7$, $s_{\max} = 0.1$, and perfect correlation between activity and attractiveness.

by their activation rates:

$$P(w) = \frac{1}{\langle a \rangle_P} \sum_{m=w}^{M} \int_{a_{\min}}^{a_{\max}} \int_{b_{\min}}^{b_{\max}} \int_{s_{\min}}^{s_{\max}} a\, p(w \mid m, s)\, p(m \mid a, b, s)\, F(a, b, s)\, da\, db\, ds, \tag{30}$$

where the summation for $m$ runs from $w$ up to the total number of RWs in the system $M$.

For a perfect correlation between activity and attractiveness, Eq. (30) reduces to

$$P(w) = \sum_{m=w}^{M} \int_{s_{\min}}^{s_{\max}} p(w \mid m, s)\, p(m \mid s)\, h(s)\, ds, \tag{31}$$

with $h(s) \sim s^{\sigma}$ and $s_{\min} = s_{\max}/N$.

The conditional probability $p(w \mid m, s)$ depends on how we define the jump process of RWs. We start by studying the Binomial model for both the small and general $s$ cases. Next, we address the Beta-Binomial model for general $s$ only.

### *1. Binomial model*

In the case of the Binomial jump model, the probability of observing $w$ RWs jumping from a node with $m$ RWs and spending rate $s$ is given by a binomial distribution, $p(w \mid m, s) = \mathrm{Bin}(m, s)$. By rearranging some terms and in the limit $M \to \infty$, Eq. (31) can be expressed as

$$P(w) = \int_{s_{\min}}^{s_{\max}} \mathcal{C}(w \mid s)\, h(s)\, ds, \tag{32}$$

where $\mathcal{C}(w \mid s)$ is a compound distribution and is defined as

$$\mathcal{C}(w \mid s) = \sum_{m=w}^{\infty} p(w \mid m, s)\, p(m \mid s). \tag{33}$$

*a. Limit of small s.* The conditional probability of observing $m$ RWs on a node with spending rate $s$ is given by the Poisson distribution, $p(m \mid s) = \mathrm{Pois}\,(\lambda_s)$. Therefore, binomial and Poisson distributions are compounded in Eq. (33), leading to

$$\mathcal{C}(w \mid s) = \sum_{m=w}^{\infty} \mathrm{Bin}(m, s)\, \mathrm{Pois}\,(\lambda_s) = \mathrm{Pois}\,(s\,\lambda_s)\,, \tag{34}$$

that is a Poisson distribution with mean $s\lambda_s$. Since $s\lambda_s = K_0$, the dependence on $s$ cancels out and Eq. (32) becomes

$$P(w) = \mathrm{Pois}\,(K_0) = \frac{(K_0)^w\, e^{-K_0}}{w!}. \tag{35}$$

*b. General s.* The conditional probability of observing $m$ RWs on a node with spending rate $s$ is given by the negative binomial distribution, $p(m \mid s) = \mathrm{NB}\left(r, \frac{r}{r+\lambda_s}\right)$, with $r$ given by Eq. (24). Therefore, binomial and negative binomial distributions are compounded in Eq. (33) now, leading to

$$\mathcal{C}(w \mid s) = \sum_{m=w}^{\infty} \mathrm{Bin}(m, s)\, \mathrm{NB}\left(r, \frac{r}{r+\lambda_s}\right) = \mathrm{NB}\left(r, \frac{r}{r+s\lambda_s}\right), \tag{36}$$

that is a negative binomial distribution with mean $s\lambda_s$. Thus, from Eq. (32) we obtain

$$\begin{aligned} P(w) &= \int_{s_{\min}}^{s_{\max}} \mathrm{NB}\left(r, \frac{r}{r+s\lambda_s}\right) h(s)\, ds \\ &\sim \frac{1}{w!} \int_{s_{\max}/N}^{s_{\max}} \frac{\Gamma\left(w + \frac{1-\langle s\rangle_h}{s}\right)}{\Gamma\left(\frac{1-\langle s\rangle_h}{s}\right)} \frac{(1-\langle s\rangle_h)^{\frac{1-\langle s\rangle_h}{s}}\,(sK_0)^w}{(1-\langle s\rangle_h + sK_0)^{\frac{1-\langle s\rangle_h}{s}+w}}\, s^{\sigma}\, ds. \end{aligned} \tag{37}$$

We evaluate this integral numerically, see Section I E.

*2. Beta-Binomial model*

In the case of the Beta-Binomial jump model, the probability of observing $w$ RWs jumping from a node with $m$ RWs and spending rate $s$ is given by a beta-binomial distribution, $p(w \mid m, s, \xi) = \mathrm{BetaBin}(m, \alpha, \beta)$, where $\alpha \equiv \xi s$ and $\beta \equiv \xi(1-s)$. Within this formulation, the mean and variance of the beta-binomial distribution are

$$\mu = ms, \qquad \sigma^2 = ms(1-s)\left(1 + \frac{m-1}{\xi+1}\right), \tag{38}$$

respectively. Thus, for $\xi \to \infty$ we recover the binomial distribution of the Binomial model.

From Section I C 2 a, the conditional probability of observing $m$ RWs on a node with spending rate $s$ is $p(m \mid s, \xi) = \mathrm{NB}\left(r_{\mathrm{eff}}, \frac{r_{\mathrm{eff}}}{r_{\mathrm{eff}}+\lambda_s}\right)$, with $r_{\mathrm{eff}}$ given by Eq. (28). In the limit $M \to \infty$, the distribution $P(w)$ of Eq. (31) reads

$$P(w) = \int_{s_{\min}}^{s_{\max}} \mathcal{C}(w \mid s, \xi)\, h(s)\, ds, \tag{39}$$

where the compound distribution is defined as

$$\begin{aligned}\mathcal{C}(w \mid s, \xi) &= \sum_{m=w}^{\infty} p(w \mid m, s, \xi)\, p(m \mid s, \xi) \\ &= \sum_{m=w}^{\infty} \mathrm{BetaBin}_w(m, \alpha, \beta)\, \mathrm{NB}_m\left(r_{\mathrm{eff}}, \frac{r_{\mathrm{eff}}}{r_{\mathrm{eff}}+\lambda_s}\right),\end{aligned} \tag{40}$$

where we used subscripts to denote the observable random variable of the distributions. Unfortunately, no closed-form solution exists for the previous expression. However, we can rely on the binomial-beta mixture representing the beta-binomial distribution,

$$\mathrm{BetaBin}_w(m, \alpha, \beta) = \int_0^1 \mathrm{Bin}_w(m, \rho)\, \mathrm{Beta}_\rho(\alpha, \beta)\, d\rho, \tag{41}$$

and the Poisson-gamma mixture representing the negative binomial distribution,

$$\mathrm{NB}_m\left(r_{\mathrm{eff}}, \frac{r_{\mathrm{eff}}}{r_{\mathrm{eff}}+\lambda_s}\right) = \int_0^{\infty} \mathrm{Pois}_m(\kappa)\, \mathrm{Gamma}_\kappa\left(r_{\mathrm{eff}}, \frac{r_{\mathrm{eff}}}{\lambda_s}\right) d\kappa, \tag{42}$$

to finally obtain

$$\begin{aligned}P(w) &= \int_{s_{\min}}^{s_{\max}} h(s)\, ds \int_0^1 \mathrm{Beta}_\rho(\alpha, \beta)\, d\rho \int_0^{\infty} \mathrm{Pois}_w(\rho\kappa)\, \mathrm{Gamma}_\kappa\left(r_{\mathrm{eff}}, \frac{r_{\mathrm{eff}}}{\lambda_s}\right) d\kappa \\ &\sim \frac{1}{w!} \int_{s_{\max}/N}^{s_{\max}} \frac{s^\sigma}{\mathrm{B}(\alpha,\beta)\Gamma(r_{\mathrm{eff}})} \left(\frac{r_{\mathrm{eff}}}{\lambda_s}\right)^{r_{\mathrm{eff}}} ds \int_0^1 \rho^{\alpha+w-1}(1-\rho)^{\beta-1}\, d\rho \int_0^{\infty} \kappa^{w+r_{\mathrm{eff}}-1}\, e^{-\left(\rho+\frac{r_{\mathrm{eff}}}{\lambda_s}\right)\kappa}\, d\kappa,\end{aligned} \tag{43}$$

where $\mathrm{B}(x, y) = \frac{\Gamma(x)\,\Gamma(y)}{\Gamma(x+y)}$ is the Beta function. We evaluate these integrals numerically, see Section I E.

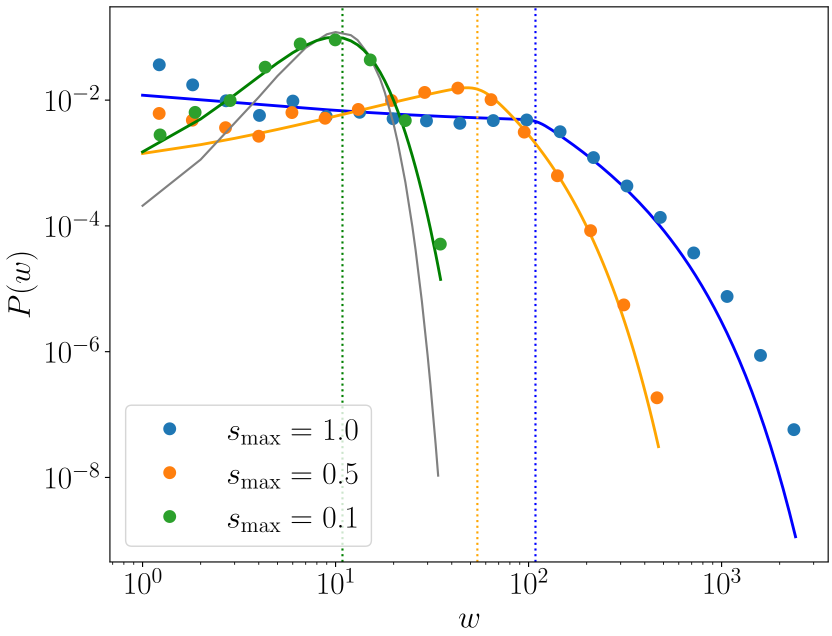


FIG. 5: Probability distribution $P(w)$ in the Binomial model for different values of maximum spending rate $s_{max}$. Solid lines correspond to numerical integrations of Eq. (37). Gray line corresponds to the analytical solution of $P(w)$ obtained under the independence assumption, see Eq. (35), shown only for small spending rates, i.e., $s_{max} = 0.1$. Vertical dotted lines correspond to $w = K_0 \approx \frac{M s_{max}}{N \ln(N)}$. We used $N = 10^4$, $M = 10^7$, $\sigma = 0$, and perfect correlation between activity and attractiveness.

### *3. Comparison with numerical simulations*

Figure 5 compares numerical simulations (points) against the distribution $P(w)$ for uniform spending rates ($\sigma = 0$) obtained numerically from Eq. (37) (solid lines) and the analytical prediction given by Eq. (35) (gray line) under the independence assumption (i.e., small $s$), for different values of $s_{max}$. One can see that the $P(w)$ distribution is recovered with very good accuracy by a numerical integration of Eq. (37), for all values of $s_{max}$. Furthermore, the analytical prediction obtained under the independence assumption provides a good approximation of the distribution for $s_{max} = 0.1$.

In Fig. 1(b) of the main text, we show that our theoretical approach for $P(w)$ also works in the Beta-Binomial model with finite $\xi$, by integrating numerically Eq. (43).

### E. Numerical integration

The integrals in Eqs. (27), (29), (37), and (43) span many orders of magnitude over the integration domain, particularly for large $m$ or $w$. Thus, standard adaptive quadrature methods widely used in numerical integration fail in this regime. Instead, we employ log-space arithmetic with the log-sum-exp trick for numerical stability [8], combined with trapezoidal integration on a log-spaced grid over the interval $[s_{\min}, s_{\max}]$.

For the integrals in Eqs. (27) and (29), to obtain $P(m)$, and in Eq. (37), to obtain $P(w)$ with $\xi = \infty$, we use $n_s = 5000$ grid points. For the multi-dimensional integral in Eq. (43), to obtain $P(w)$ at finite $\xi$, we use $n_\kappa = 100$ points (log-spaced, centered on $\lambda_s$) and $n_\rho = 50$ points (linearly spaced on $(0, 1)$), with an outer integral over $s$ using $n_s = 200$ points.

The implementation uses NumPy [9] and SciPy [10] for array operations and special functions. Code files were written by Claude AI (Anthropic) and are available in the supplementary repository at https://github.com/carolinamattsson/transactions.

## II. EMPIRICAL DATA

### A. Data description

The Sarafu dataset records digital transactions within a complementary currency system in Kenya. The dataset, available on *UK Data Service*'s portal [11], includes anonymized account information for approximately 55,000 users and a record of approximately 940,000 transactions covering the period from January 25, 2020, to June 15, 2021. These transactions, totaling around 300 million Sarafu in exchanged volume (approximately 2.8 million USD), capture a range of economic activities, including peer-to-peer trade, savings group contributions, and participation in local economic networks known as *Chamas.*

The Sarafu dataset consists of two main datasets: the `transaction dataframe` and the `user dataframe`, which we denote by $\mathcal{T}$ and $\mathcal{U}$, respectively. The attributes that characterize transactions are the following:

- Timestamp: $t \in [t_0, t_f]$, the moment in time the transaction took place.
- Source and target: $(s, r) \in \{1, ..., V\}$, the sender and the recipient of the transactions.
- Weight: $w \in \mathbb{R}^+$, the amount of money that was transferred in the transaction.
- Type: $c$, the category of transactions.

There are 4 categories of transactions:

- STANDARD, represents the flow of money from a non-administrative user to another. These transactions represent those we are interested in.
- DISBURSEMENT, adds Sarafu to an account, represents currency creation.
- RECLAMATION, removes Sarafu from an account, represents money destruction.
- AGENT OUT, cash exchange operation, represents currency destruction.

Figure 6 shows the weekly total number of transactions per type. As one can see, the number of transactions is not steady over time, with different transaction types being very heterogeneous. To assess the significance of fluctuations in weekly activity on total balance, we define:

- $\mathcal{D}$: the sum of disbursements.
- $\mathcal{S}$: the sum of standard transactions.
- $\mathcal{O}$: the sum of reclamations and withdrawals.
- $\mathcal{N} = \mathcal{D} - \mathcal{O}$: the net flow through the system.
- $\mathcal{B}$: the sum of all balances.

We measure each quantity at 20 different timestamps. Figure 7(a) shows that the net flow takes both positive and negative values, meaning that there are inflations and contractions in the total balance within the system. However, the total volume circulating in the system is, in most cases, much larger than the volume flowing into or out. Therefore, in- and out-flows are negligible with respect to the amount of standard transactions.

Figure 7(b) shows the number of users (population size), the total balance, and the number of transactions over time, rescaled in the interval $[0, 1]$. The number of registered accounts grows from 8,354 to around 55,000 during the observation period. One can see that both the system (number of users) and the amount of Sarafu deposited (balance) grow in size, while the activity on the network (number of transactions of any kind) grows in the first instance and declines thereafter.

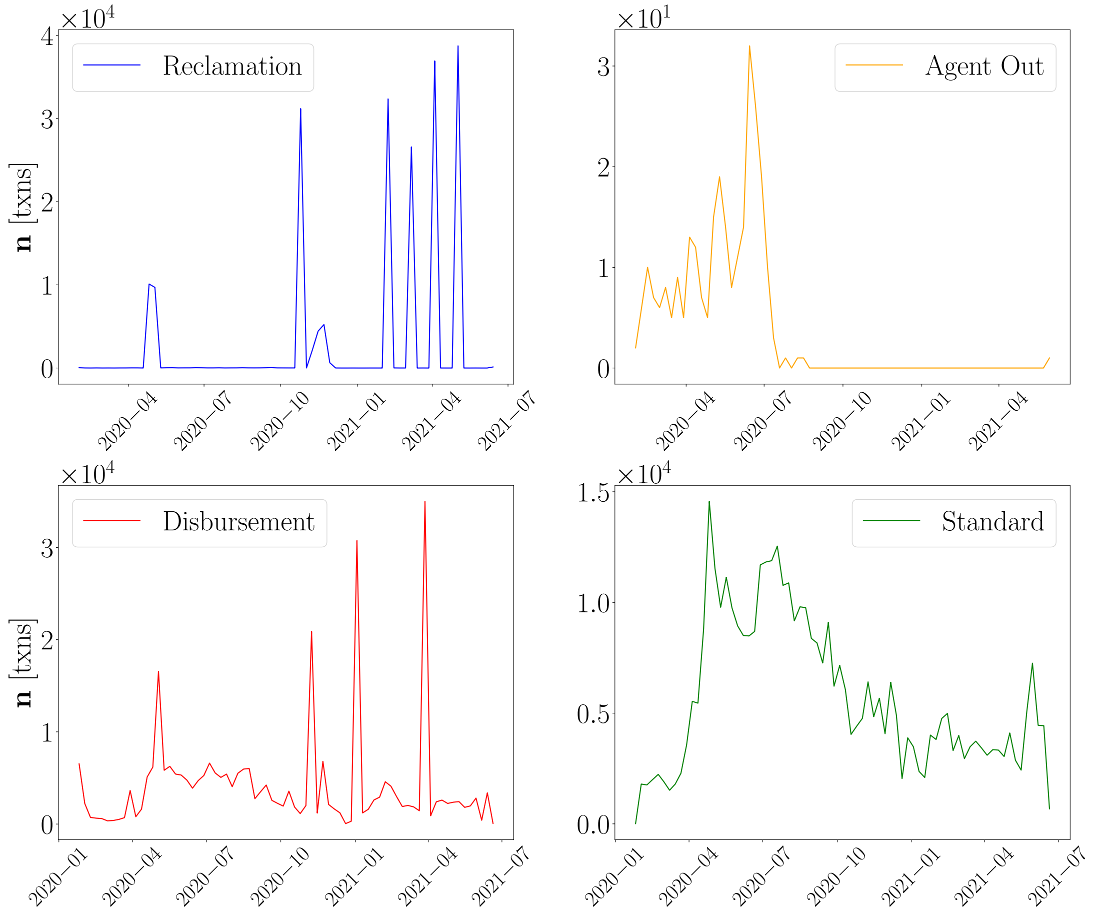


FIG. 6: Weekly activity for different transaction types in the Sarafu dataset. STANDARD, DISBURSEMENT, RECLAMATION, AGENT OUT. The fluctuations over time highlight changing economic activity within the system.

### B. Balance reconstruction

The dataset has been thoroughly investigated in Refs. [12, 13], supporting its reliability and quality. However, one limitation is that the transaction records do not include the balance of accounts (the amount of Sarafu owned by a user at a certain time). Balance information is necessary to define the fraction of the balance that users spend at each transaction, to reconstruct the spending rates of users in the model. Therefore, we reconstruct the balances. While Ref. [12] assumed an initial zero balance and validated the reconstructed balances by comparing the final state with the `final_bal` column, we adopt a different strategy. Given that the initial balance is unknown, we instead use the final balance as a reference point and reconstruct past balances by working backward in time. As a result, only four users (representing only 0.007%) exhibit a reconstructed final balance that is inconsistent with the corresponding value provided in the dataset, confirming the overall reliability of the data. These users are

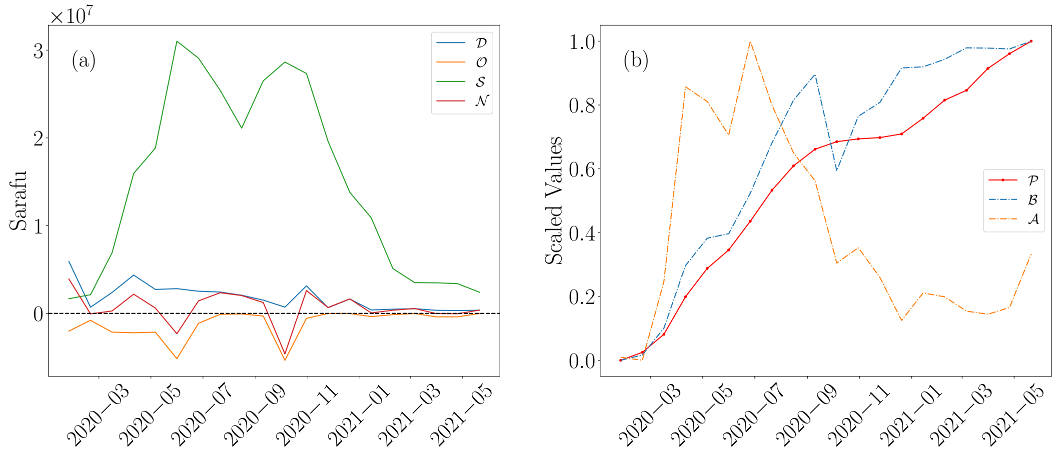


FIG. 7: System-level properties. Panel (a) reports the main monetary flows in the system: inflows due to money creation ($\mathcal{D}$), outflows due to reclamations and withdrawals ($\mathcal{O}$), internal circulation through standard transactions ($\mathcal{S}$), and the resulting net flow ($\mathcal{N} = \mathcal{D} - \mathcal{O}$). Panel (b) compares, on a normalized scale, population size ($\mathcal{P}$), total balances ($\mathcal{B}$), and overall transactional activity ($\mathcal{A}$).

excluded from the subsequent analysis.

### C. Filtering and preprocessing

We filter the dataset by selecting certain user types, transaction types, a minimum transaction size, and users with a minimum number of transactions. The final dataset consists of 23,735 users (accounting for 43% of the original dataset) and 388,609 transactions (42% of the original dataset).

*a. User type.* We focus on transactions conducted by users classified as {"VENDOR", "BENEFICIARY", "GROUP ACCOUNT"}, excluding administrative accounts. This subset, referred to as *standard users*, constitutes 99% of the entire population and serves as the foundation of our analysis. Additionally, we exclude transaction records from accounts with unverified balance histories.

*b. Transaction type.* The only kind of transactions considered for our purposes is the "STANDARD", since they are not related to money creation or dissolution. Except for rare cases, these transactions involve solely users of a non-administrative type. STANDARD transactions represent the 45% of the total transactions recorded.

*c. Minimum transaction size.* We select only transactions in which at least 1 Sarafu has been exchanged. Since 1 Sarafu is approximately 1 Kenyan Shilling, this threshold filters

out very small transactions, accounting for just 0.01% of the total number of STANDARD transactions. In 2021, the Kenyan Shilling (KES) experienced fluctuations with respect to the US Dollar (USD), with an average exchange rate of approximately 1 USD $\approx$ 109.9 KES (`www.exchangerates.org.uk/KES-USD-spot-exchange-rates-history-2021.html`). The purchasing power parity (PPP) conversion factor for Kenya was approximately 46.41 KES per international dollar. Given that the average market exchange rate was around 109.68 KES per USD, the PPP conversion factor suggests that the Kenyan Shilling had a higher purchasing power within Kenya than the market exchange rate indicated. Specifically, 1 KES could buy goods and services in Kenya equivalent to what approximately 2.36 cents (USD) could purchase in the United States (`www.indexmundi.com/facts/kenya/ppp-conversion-factor`).

*d. Minimum number of transactions.* We retain only users who have both sent and received at least one transaction.

## D. Statistical properties

In this Section, we present some statistical properties of the Sarafu dataset.

### *1. Activity and attractiveness*

For each user, we record two key quantities: The number of transactions they initiated and the number of transactions they received, denoted by $n_i^{\text{out}}$ and $n_i^{\text{in}}$, respectively. The motivation behind these measurements stems from their direct connection to the probability that a randomly selected agent either sends or receives a transaction.

*a. Marginal distributions.* The empirical distributions of these two quantities, shown in Figure 8, exhibit striking similarities in both shape and range.

We utilize the `powerlaw` Python package for analyzing heavy-tailed distributions [14, 15]. For simplicity, we assume a power-law distribution and estimate its parameters. To optimize the power-law exponent parameter, we employ Maximum Likelihood Estimation (MLE). The `powerlaw` library provides an optimization criterion based on the Kolmogorov–Smirnov (KS) test to determine the lower bound $x_{\text{min}}$. However, using this criterion leads to a very high fit for attractiveness, where the power-law behavior is observed only in the extreme upper tail. Instead, we adopt a percentile-based criterion for selecting $x_{\text{min}}$. Specifically, we set $x_{\text{min}}$ such that at least 80% of the data points are above $x_{\text{min}}$. To assess the fit quality, we compute the Jensen–Shannon distance (JSD), which represents a symmetric measure of similarity between distributions bounded within the interval $[0, \ln(2)]$. Our approach involves: Sampling from the

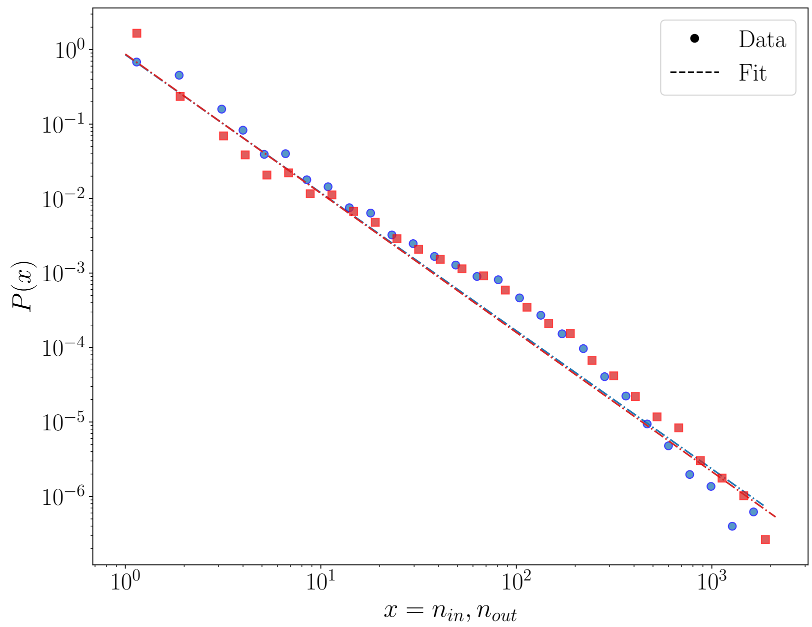


FIG. 8: Empirical distributions of the number of outgoing ($n_{\text{out}}$, blue points) and ingoing ($n_{\text{in}}$, red points) transactions per user, with corresponding power-law fits (dashed lines). For outgoing transactions, the lower cutoff is $x_{\text{min}} = 2.0$ with a Kolmogorov–Smirnov statistic of 0.0435, and the fit is estimated from the upper 80.61% of the data. For ingoing transactions, the cutoff is $x_{\text{min}} = 1.0$, the Kolmogorov–Smirnov statistic is 0.0811, and the fit uses the full dataset (100%). The fitted power-law exponents $\alpha$ are reported for both distributions in Table I.

| | **Activity** | **Attractiveness** |
|---|---|---|
| $\alpha$ | 1.85 | 1.87 |
| $x_{\text{min}}$ | 2 | 1 |
| $x_{\text{max}}$ | 1883 | 2187 |
| JSD | 0.09 | 0.07 |

TABLE I: Power-law fit parameters for activity and attractiveness.

fitted distribution, ensuring that the number of data points and the range remain consistent with respect to the original dataset, and finally computing the JSD between the empirical and sampled distributions. The estimated parameters and goodness-of-fit measures for the power-law distribution fit to activity ($n_{\text{out}}$) and attractiveness ($n_{\text{in}}$) are summarized in Table I. One can see that the computed JSD indicates a discrepancy of nearly 10%, which is acceptable given our assumptions and the limitations of the power-law model.

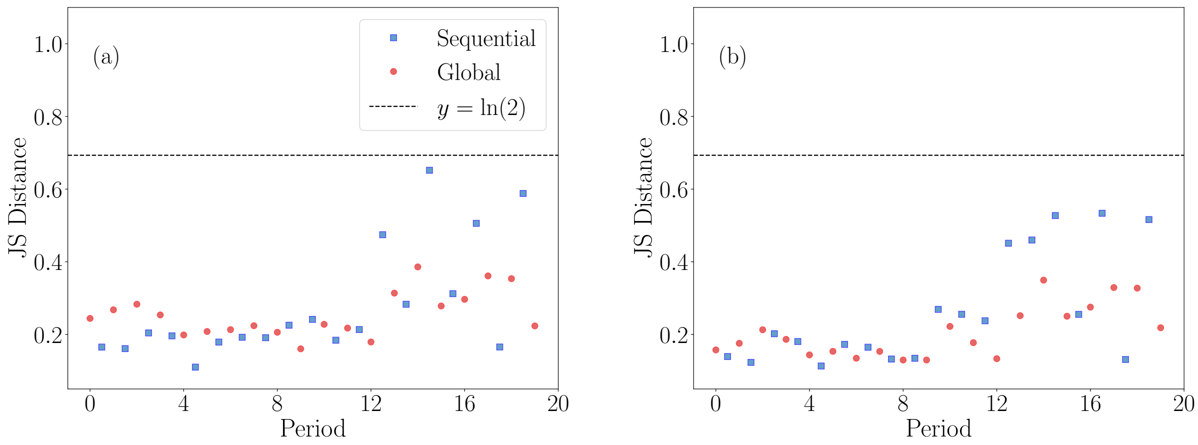


FIG. 9: Jensen–Shannon distance (JSD) of transaction distributions over time, blue points for sequential measure, red points for global measure. Panel (a) shows the stationarity test for incoming transactions, $n_{\text{in}}$. Panel (b) shows the stationarity test for outgoing transactions, $n_{\text{out}}$. The horizontal dashed line represents the ceiling value $\ln(2)$.

*b. Evolution over time.* To address the variability of these distributions over time, we compute the Jensen–Shannon distance (JSD). To do so, we divide the transaction record into 20 periods, each one containing the same number of transactions, meaning that the actual duration in time of periods is similar. In each period, an estimate of the empirical distributions is given, and then the JSD is measured in two ways:

- Sequential measure: we calculate the distance between two consecutive periods

$$\mathrm{JSD}(P_t(n), P_{t-1}(n)).$$

- Global measure: we calculate the distance between the distribution recorded at period $t$ and the distribution observed over the whole time span

$$\mathrm{JSD}(P_t(n), P(n)).$$

The results, displayed in Figure 9, show that the distributions slightly vary over time, yet the scores are consistently far away from the ceiling value $\ln(2)$. We can assume these effects are noise-generated effects, but the distribution functional form remains steady. Figure 10 shows that the distributions of incoming and outgoing transactions, $P(n_{\text{in}})$ and $P(n_{\text{out}})$, respectively, have a very similar functional form when reconstructed over different time windows. Therefore, the activity and attractiveness distributions are stationary over time. This crucial assumption allows us to use the integrated distributions and sample features of agents in our model.

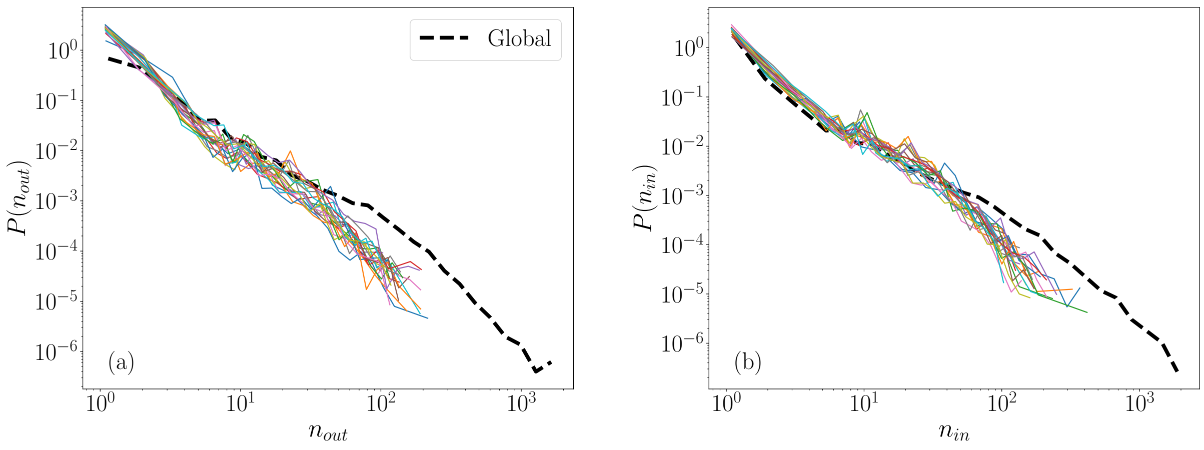


FIG. 10: Empirical distributions of the number of outgoing [$n_{\text{out}}$, (a)] and incoming [$n_{\text{in}}$, (b)] transactions per user, reconstructed over different time windows (different colors). The black dashed line represents the global distribution reconstructed over the whole time window.

*c. Correlation between activity and attractiveness.* We also examine the correlation between activity and attractiveness. As shown in Figure 11, there is a clear positive correlation between $n_i^{\text{in}}$ and $n_i^{\text{out}}$, which is quantitatively confirmed by the Pearson correlation coefficient $\rho \approx 0.7$. The data visualization further highlights this relationship, with color intensity determined by the non-parametric estimate of the probability density measured through Kernel Density Estimation (KDE) (we employed the `gaussian_kde` Python module in `scipy.stats` [10]). The majority of users cluster in the lower-value region, where the data points form a square-like pattern, indicating that, in this range, $n_i^{\text{in}}$ and $n_i^{\text{out}}$ are largely uncorrelated. By contrast, the correlation appears much more pronounced in the high-valued region, suggesting that more active users are also more likely to be targeted.

### *2. Inter-event time distribution between consecutive transactions*

We measure the inter-event time distribution $P(\tau)$ between consecutive transactions of a single user, i.e., the time $\tau$ elapsed between two consecutive transactions performed by the same user. Figure 12 shows the inter-event time distributions of the ten most active users, together with the inter-event time distribution over the whole population (i.e., by aggregating over all users). One can see that the transaction dynamics is bursty, i.e., users perform transactions by following a non-Poissonian process. Therefore, in the model, we simulate activation events by using a Weibull distribution with a small parameter $k$. Furthermore, the individual $P(\tau)$ distributions are very similar across users. This justifies the choice of a unique global inter-event

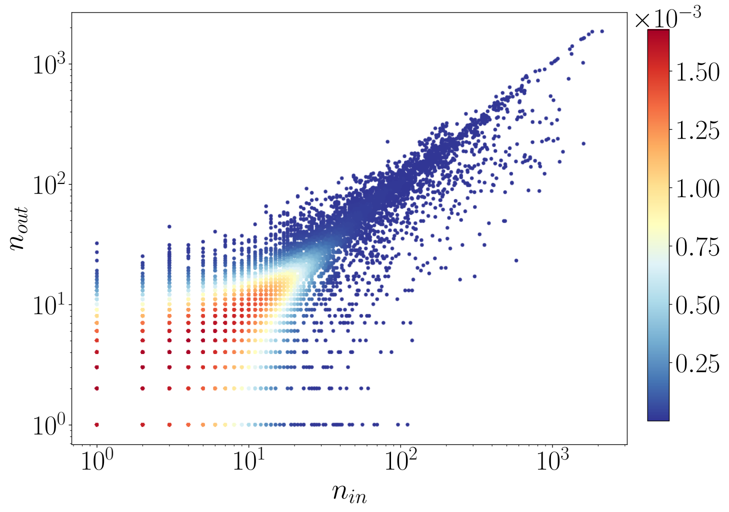


FIG. 11: Correlation structure of $n_{\rm in}$ and $n_{\rm out}$. Color represents probability density.

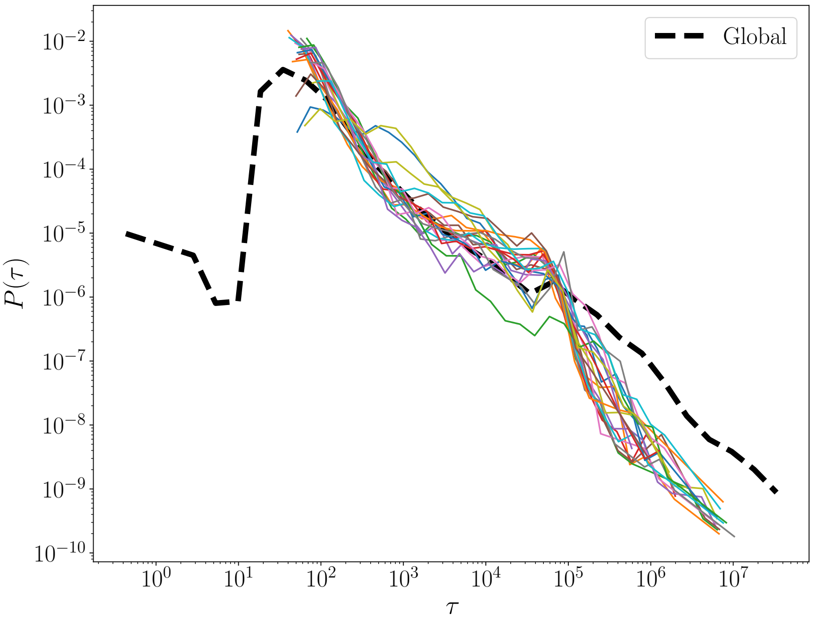


FIG. 12: Inter-event time distributions of the ten most active individuals from the Sarafu dataset, shown in colored solid lines. For reference, the global inter-event time distribution measured at the population level is shown in black dashed line.

time distribution with a single level of burstiness in the model.

## III. MODEL CALIBRATION

### A. Correlation between activity and attractiveness

The Sarafu dataset exhibits a strong correlation between activity and attractiveness of a node, i.e., the number of outgoing and incoming transactions ($n_{\text{out}}$ and $n_{\text{in}}$, respectively), whereby more active nodes are also more likely to receive more transactions. To model this dependence, we use bivariate copulas. Let $(u, v)$ be a random sample drawn from a fitted copula $C$. To map this pair into the data space of activity $X$ and attractiveness $Y$, we apply inverse transform sampling using the empirical or parametric marginal distributions $F_X$ and $F_Y$, that is $x = F_X^{-1}(u)$ and $y = F_Y^{-1}(v)$. The resulting pair $(x, y)$ has marginals $F_X, F_Y$ and dependence structure induced by the copula $C$, providing a synthetic observation consistent with the empirical activity-attractiveness joint distribution, $P(a, b)$.

We estimate copula parameters using Canonical Maximum Likelihood Estimation (CMLE) implemented in the `pycop` Python library. Among the tested models, the Joe copula provides the best fit, with estimated parameter $\theta \approx 3.15$:

$$C_\theta(u, v) = 1 - \Big((1-u)^\theta + (1-v)^\theta - (1-u)^\theta(1-v)^\theta\Big)^{1/\theta}, \qquad \theta \geq 1, \tag{44}$$

which exhibits upper-tail dependence for $\theta > 1$. To validate the fit, we draw a bivariate sample $(u, v)$ from the fitted copula and compare its kernel density with a jittered rank of outgoing and incoming transactions, $n_{\text{out}}$ and $n_{\text{in}}$, in the Sarafu dataset, see Figure 13. To obtain the jittered rank, we apply a simple uniformly distributed perturbation $\varpi \sim \mathcal{U}_{[0,1]}$ to the ranks, which helps with visualization. In Figure 14 we directly compare the resulting activity-attractiveness joint distribution, $P(a, b)$, of the empirical copula with the one observed in the Sarafu dataset.

One can see that the copula provides a good approximation of the observed dependence pattern. We further compare Pearson, Kendall, and Spearman correlations of ranked data and jittered ranks with the copula sample, see Table II. Pearson and Spearman coefficients of the copula sample closely match those of ranked data, while Kendall's lies between the ranked and jittered estimates, supporting the adequacy of the fitted Joe copula.

### B. Non-Poissonian activation dynamics

Non-Poissonian activation in continuous-time activity-driven networks is modeled by replacing memoryless Poisson processes with renewal processes. This approach allows us to capture empirical features such as burstiness. A renewal process $\{N(t),\, t \geq 0\}$ is a counting process where the inter-event times $\{\tau_1, \tau_2, \ldots\}$ are independent and identically distributed (i.i.d.) with

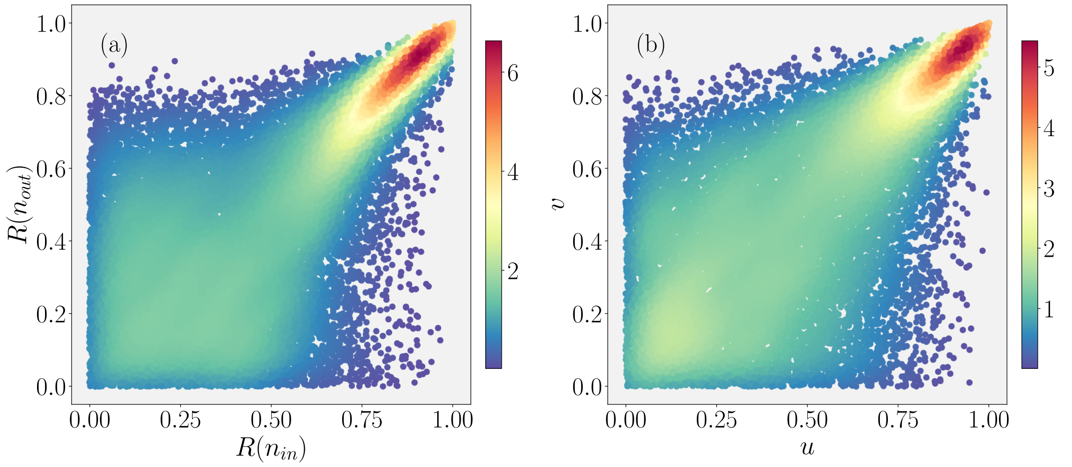


FIG. 13: Probability density of the jittered ranks $R(n_{\rm out})$ and $R(n_{\rm in})$ (a), and of the copula sample $(u, v)$ (b). Each point in panel (a) corresponds to a user in the Sarafu dataset, while each point in panel (b) corresponds to the input of a model agent.

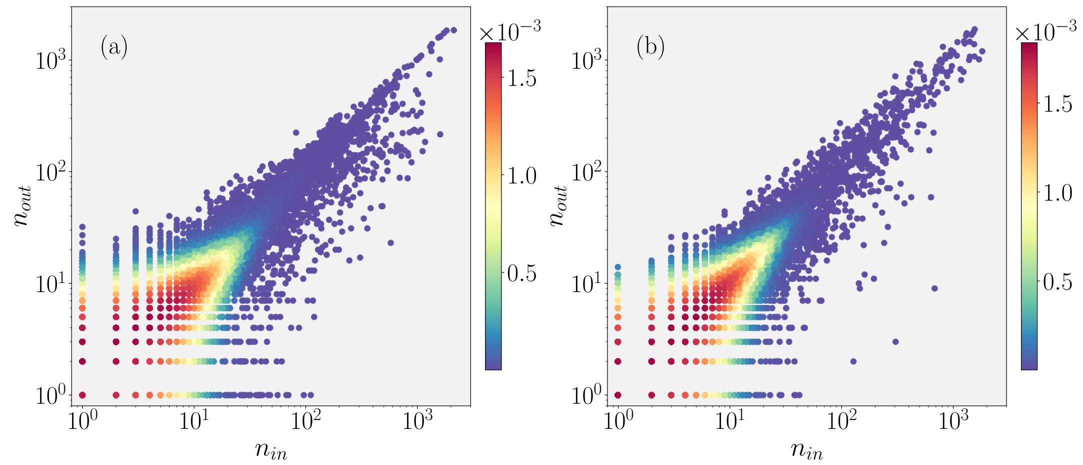


FIG. 14: Activity-attractivess patterns observed in the Sarafu dataset (a) and in the Beta-Binomial model with $\xi = 1$ and $k = 0.75$ (b). One point corresponds to one agent. Color represents probability density of agents, and density has been estimated through Kernel Density Estimation. Note that panel (a) is the same as Figure 11.

| | **Ranks** | **Jittered Ranks** | **Copula sample** |
|---|---|---|---|
| **Pearson** | 0.73 | 0.68 | 0.73 |
| **Kendall** | 0.62 | 0.51 | 0.54 |
| **Spearman** | 0.73 | 0.68 | 0.72 |

TABLE II: Correlation coefficients of ranked Sarafu ($n_{\rm out}$, $n_{\rm in}$) without and with jittering and of the Joe copula sample.

a cumulative distribution function $F_\tau(t)$. The *renewal function* $\mathcal{M}(t) = \mathbb{E}[N(t)]$ represents the mean number of events expected up to time $t$. If the mean inter-event time $\mathbb{E}[\tau]$ is finite, the Elementary Renewal Theorem implies that the long-term rate of events converges to the reciprocal of the mean:

$$\mathcal{M}(t) \sim \frac{t}{\mathbb{E}[\tau]}, \qquad t \to \infty.$$

*a. The Weibull renewal model.* We model the node activations using a Weibull distribution, which generalizes the exponential distribution to accommodate bursty dynamics. The inter-event time probability density function (PDF) with shape $k > 0$ and scale $\ell > 0$ is

$$f(\tau; k, \ell) = \frac{k}{\ell}\left(\frac{\tau}{\ell}\right)^{k-1} \exp\left[-\left(\frac{\tau}{\ell}\right)^{k}\right], \qquad \tau \geq 0.$$

The mean inter-event time for this distribution is $\mathbb{E}[\tau] = \ell\,\Gamma(1 + 1/k)$. Consequently, for large $t$, the expected number of events is

$$\mathcal{M}(t) \sim \frac{t}{\ell, \Gamma(1 + 1/k)}. \tag{45}$$

When $k = 1$, the Weibull distribution reduces to the exponential distribution, recovering the standard Poisson process. Values of $k < 1$ indicate "bursty" behavior (decreasing hazard rate), while $k > 1$ indicates regular behavior.

*b. Application to activity-driven networks.* In our continuous-time network model, each node $i$ operates as an independent renewal process. We assign each node an empirical activity rate $a_i = x_i/T$, where $x_i$ is the node's total number of events (sampled from a power-law distribution with exponent 1.85) and $T$ is the observation window. To ensure that each node $i$ maintains its specific average activity rate $a_i$ while exhibiting burstiness governed by a global shape parameter $k$, we set the node-specific scale parameter $\ell_i$ such that the theoretical rate matches the empirical rate ($1/\mathbb{E}[\tau] \approx a_i$). Using Eq. (45), this yields

$$\ell_i = \frac{1}{a_i, \Gamma(1 + 1/k)}. \tag{46}$$

This parameterization allows us to tune the burstiness of the network via $k$ while preserving the heterogeneous activity levels observed in the data.

## IV. ADDITIONAL RESULTS FROM THE MODEL

### A. Robustness of the model to $k$ and $\xi$

We show the balance distribution $P(m)$ and the transaction size distribution $P(w)$ obtained from simulations of the model, for different values of $k$ (Poissonian vs non-Poissonian activation patterns) and $\xi$ (Binomial and Beta-Binomial dynamics).

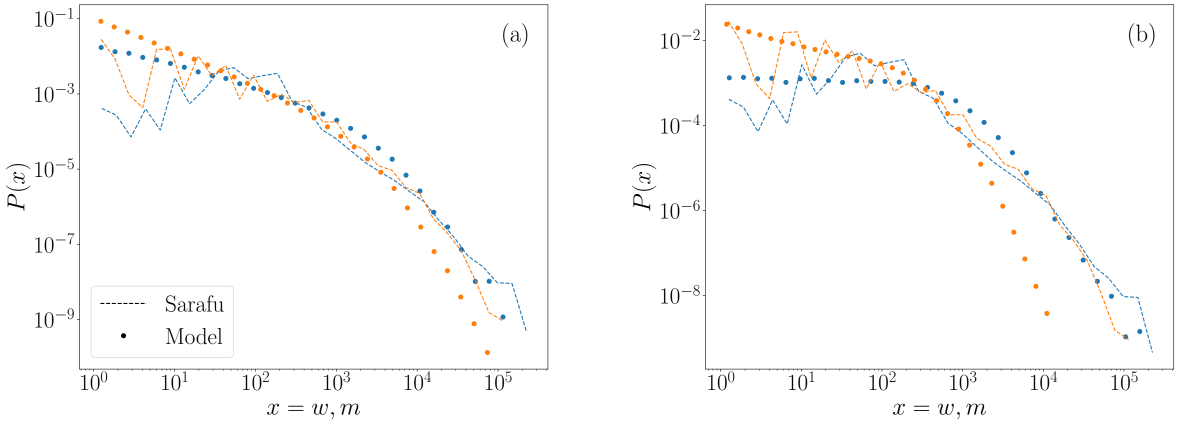


FIG. 15: Probability distributions of balances $P(m)$ (blue) and transaction sizes $P(w)$ (orange), observed in the data (dashed lines) and obtained from simulations (points) of the Beta-Binomial model without burstiness $\xi = 1$, $k = 1$ (a) and with high precision $\xi = 250$, $k = 1$ (b). 1 Sarafu from data corresponds to 1000 RWs in the simulation.

From Fig. 2 of the main text, we observe that the model is able to reproduce the $P(m)$ and $P(w)$ distributions for low spending dispersion ($\xi = 1$) and for a non-Poissonian process, i.e., $k < 1$. Figure 15(a) shows that both distributions are also reproduced for a Poissonian process, i.e., $k = 1$. Therefore, the activation dynamics does not play an important role in the model behavior. However, Figure 15(b) shows that the model is able to reproduce $P(m)$ for high spending precision ($\xi = 250$), but not $P(w)$. A heterogeneous spending behavior of individuals, thus, is responsible for the heavy-tailed nature of the transaction size distribution.

Finally, Figure 16 shows that the model properly reproduces the distributions of average balance $\langle m \rangle$ and average transaction size $\langle w \rangle$ per individual, for any values of $\xi$ and $k$.

### B. Degree distribution

Figure 17 shows that the model is able to reproduce the distributions of in-degree and out-degree observed in the data, $k_{\text{in}}$ and $k_{\text{out}}$, respectively, for different values of the precision parameter $\xi$.

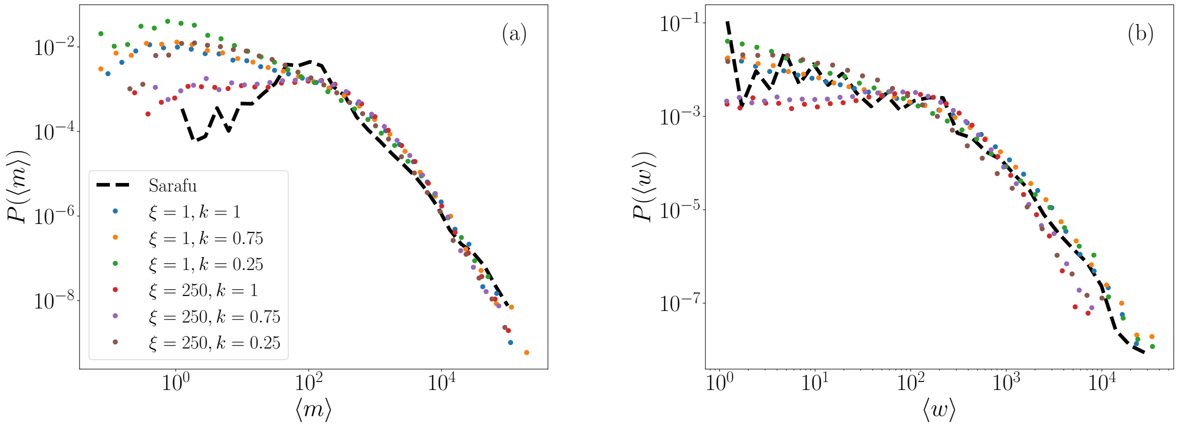


FIG. 16: Probability distributions of the average balance $\langle m \rangle$ (a) and average transaction size $\langle w \rangle$ (b) per individual, for different values of $\xi$ and $k$. Average balances are computed by averaging 20 balance observations per user over the full time span. Average transaction sizes are obtained by averaging, for each user, the sizes of all transactions performed over the full time span.

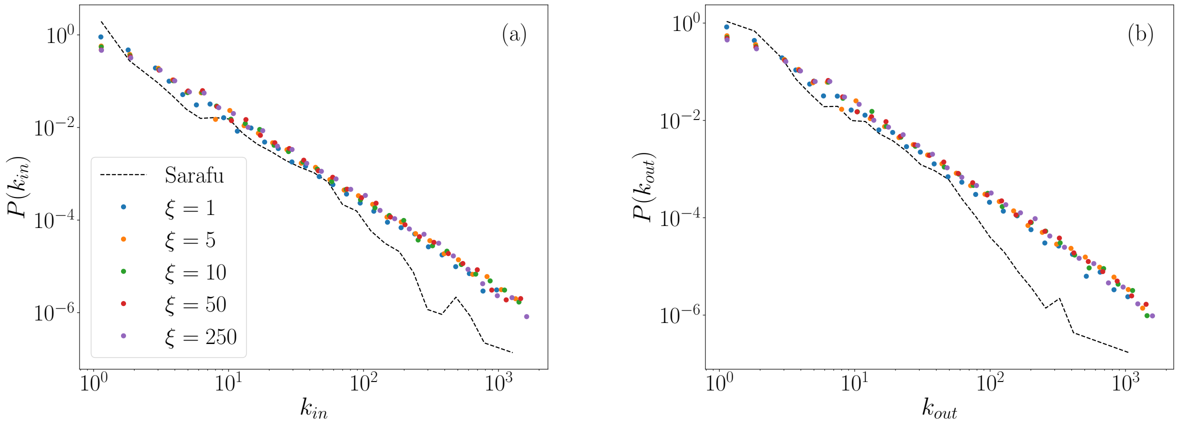


FIG. 17: Probability distribution of the in-degree $P(k_{\text{in}})$ (a) and out-degree $P(k_{\text{out}})$ (b), observed in the data (dashed line) and obtained from simulations of the Beta-Binomial model for different values of $\xi$ and $k = 0.75$ (points). $k_{\text{out}}$ and $k_{\text{in}}$ have been measured as the total number of unique target nodes and source nodes for each individual, respectively.

[1] M. Abramowitz and I. A. Stegun, *Handbook of mathematical functions.* (Dover, New York, 1972).

[2] D. A. Williams, Biometrics **31**, 949 (1975).

[3] N. L. Johnson, A. W. Kemp, and S. Kotz, *Univariate Discrete Distributions*, 1st ed., Wiley Series in Probability and Statistics (Wiley, 2005).

[4] M. Patriarca, E. Heinsalu, and A. Chakraborti, Eur. Phys. J. B **73**, 145 (2010).

[5] S. Ispolatov, P. L. Krapivsky, and S. Redner, Eur. Phys. J. B **2**, 267 (1998).

[6] J. Angle, The Journal of Mathematical Sociology **26**, 217 (2002).

[7] J. Angle, Physica A: Statistical Mechanics and its Applications **367**, 388 (2006).

[8] P. Blanchard, D. J. Higham, and N. J. Higham, IMA J Numer Anal **41**, 2311 (2021).

[9] C. R. Harris, K. J. Millman, S. J. van der Walt, R. Gommers, P. Virtanen, D. Cournapeau, E. Wieser, J. Taylor, S. Berg, N. J. Smith, R. Kern, M. Picus, S. Hoyer, M. H. van Kerkwijk, M. Brett, A. Haldane, J. F. del Río, M. Wiebe, P. Peterson, P. Gérard-Marchant, K. Sheppard, T. Reddy, W. Weckesser, H. Abbasi, C. Gohlke, and T. E. Oliphant, Nature **585**, 357 (2020).

[10] P. Virtanen, R. Gommers, T. E. Oliphant, M. Haberland, T. Reddy, D. Cournapeau, E. Burovski, P. Peterson, W. Weckesser, J. Bright, S. J. van der Walt, M. Brett, J. Wilson, K. J. Millman, N. Mayorov, A. R. J. Nelson, E. Jones, R. Kern, E. Larson, C. J. Carey, İ. Polat, Y. Feng, E. W. Moore, J. VanderPlas, D. Laxalde, J. Perktold, R. Cimrman, I. Henriksen, E. A. Quintero, C. R. Harris, A. M. Archibald, A. H. Ribeiro, F. Pedregosa, P. van Mulbregt, and SciPy 1.0 Contributors, Nature Methods **17**, 261 (2020).

[11] W. O. Ruddick, Sarafu Community Inclusion Currency, 2020-2021 (2021).

[12] C. E. S. Mattsson, T. Criscione, and W. O. Ruddick, Sci Data **9**, 426 (2022).

[13] C. E. S. Mattsson, T. Criscione, and F. W. Takes, Sci Rep **13**, 5864 (2023).

[14] J. Alstott, E. Bullmore, and D. Plenz, PLOS ONE **9**, e85777 (2014).

[15] A. Clauset, C. R. Shalizi, and M. E. J. Newman, SIAM Review **51**, 661 (2009).
